# Supplementary material for: Synthesizing Conjunctive Queries for Code Search
Source: arXiv:2305.04316 source file (2023-05-11)
Supplement: Supplementary file 1 [file appendix.tex]

We present several examples of method semantic specification and complexity specification.
In the implementation of \ToolName, we provide the specifications of all the container methods in a configuration file,
and we only list several typical examples as follows.

In the supplementary material, we discuss container methods along with their parameter types to distinguish the methods with the same method names.
For example, there are two methods named \textsf{add} in \textsf{ArrayList}, which insert an element at the end of the list and at the specific position, respectively.
We indicate the methods by \textsf{ArrayList.add(O)} and \textsf{ArrayList.add(I, O)} to distinguish them.
In the paper, we just omit the parameter types of the methods in the examples to simplify the illustration.

\section{Method Semantic Specification}
We consider three container types as examples, including \textsf{ArrayList}, \textsf{HashSet}, and \textsf{LinkedHashMap}.

\subsection{Container-Property Queries}
$\ $\\
The set of container-property queries $\mathcal{Q}$ contains the following queries:
\begin{itemize}[leftmargin=*]
	\item $\textsf{size}:=\textsf{q-size}(c, s)$ indicates the size of the container object, i.e.,
	$$\textsf{size} = |\{ \lambda \ | \ (\varepsilon(c), \ \lambda) \in dom(\mu)\}|$$
	\item $\textsf{isIdx}(\lambda):=\textsf{q-isIdx}(c, s)$ indicates whether a value $\lambda$ is an index in $c$, i.e.,
	$$\textsf{isIdx}(\lambda) = ite((\varepsilon(c), \lambda) \in dom(\mu), T, F)$$
	Similarly, $\textsf{isVal}(v):=\textsf{q-isVal}(c, s)$ indicates whether a value $v$ is a value stored in $c$, i.e.,
	$$\textsf{isVal}(v) = ite(\exists \lambda\  \mu(\varepsilon(c), \lambda) = v, T, F)$$
	\item $\textsf{isCor}(\lambda, v):=\textsf{q-isCor}(c, s)$ indicates whether a value $v$ stored in $c$ is paired with the index $\lambda$, i.e.,
	$$\textsf{isCor}(\lambda, v) = ite(\mu(\varepsilon(c), \lambda)=v, T, F)$$
	\item $\textsf{InsOrd}(\lambda_{1}, \lambda_{2}):=\textsf{q-InsOrd}(c,s)$ indicates whether a key $\lambda_{1}$ is inserted before the other key $\lambda_{2}$, i.e., 
	$$\textsf{InsOrd}(\lambda_{1}, \lambda_{2}) = ite(\lambda_{1} \preceq \lambda_{2}, T, F)$$
	where $\preceq$ is the insertion order of the keys.
\end{itemize}
To sum up, we can construct a family of container-property queries $$\mathcal{Q}=\{\textsf{q-size}, \textsf{q-isIdx}, \textsf{q-isVal}, \textsf{q-isCor}, \textsf{q-InsOrd}\}$$

\subsection{Container-Property Modifiers}
$\ $\\
The set of container-property modifiers $\mathcal{T}$ contains the following modifiers, 
which can be categorized into five types.
\begin{itemize}[leftmargin=*]
	\item Size modifiers can increase or decrease the size of the container object by one or at most one.
	We denote them by $\textsf{t-size}_{+}^{=1}$, $\textsf{t-size}_{-}^{=1}$, $\textsf{t-size}_{+}^{\leq 1}$, and $\textsf{t-size}_{-}^{\leq 1}$, respectively.
	\item Index-ownership modifiers can add an index to the container or remove an index from the container if it exists.
	We denote them by $\textsf{t-idx}_{+}$ and $\textsf{t-idx}_{-}$, respectively.
	\item Value-ownership modifiers can add a value to the container or remove an value from the container if it exists.
	We denote them by $\textsf{t-val}_{+}$ and $\textsf{t-val}_{-}$, respectively.
	\item Correlation modifiers can change index-value correlation of a list object in six ways, including inserting/removing an element at the beginning/end/specific position.
	We denote them by $\textsf{t-cor}_{+}^{b}$, $\textsf{t-cor}_{-}^{b}$, $\textsf{t-cor}_{+}^{e}$, $\textsf{t-cor}_{-}^{e}$, $\textsf{t-cor}_{+}^{p}$, and $\textsf{t-cor}_{-}^{p}$, respectively.
	Similarly, correlation modifiers can change index-value correlation of a map object in two ways, including inserting/removing a key-value pair with a specific key.
	We denote them by $\textsf{t-cor}_{+}^{k}$ and $\textsf{t-cor}_{-}^{k}$, respectively.
	\item Insertion-order modifiers change the insertion order of a container object in two ways, including adding an index as the largest element in the partial order set, and removing an index from the partial order set.
	We denote them by $\textsf{t-InsOrd}_{+}$ and $\textsf{t-InsOrd}_{-}$, respectively.
\end{itemize}

To sum up, we can construct a family of container-property modifiers 
\begin{align*}
\mathcal{T}=\{
&\textsf{t-size}_{+}^{=1},\ \textsf{t-size}_{-}^{=1}, \ \textsf{t-size}_{+}^{\leq 1},\ \textsf{t-size}_{-}^{\leq 1},\\
&\textsf{t-idx}_{+}, \ \textsf{t-idx}_{-}, \textsf{t-val}_{+}, \ \textsf{t-val}_{-},\\
&\textsf{t-cor}_{+}^{b}, \ \textsf{t-cor}_{-}^{b}, \ \textsf{t-cor}_{+}^{e}, \ \textsf{t-cor}_{-}^{e}, \ \textsf{t-cor}_{+}^{p}, \ \textsf{t-cor}_{-}^{p}, \\
&\textsf{t-cor}_{+}^{k}, \ \textsf{t-cor}_{-}^{k},\\
&\textsf{t-InsOrd}_{+}, \ \textsf{t-InsOrd}_{-}
\}
\end{align*}

At last, we can define $\omega_{\mathcal{T}}$ according to Table~\ref{table:omega}.
Each row shows the affected container-property queries of a specific container-property modifier.

\begin{table}[t]
	\centering
	\caption{Definition of $\omega_{\mathcal{T}}$.}
	\resizebox{0.6\linewidth}{!} 
	{
		\begin{tabular}{c|ccccc}
		\toprule
			& \textsf{q-size} & \textsf{q-isIdx} & \textsf{q-isVal} & \textsf{q-isCor} & \textsf{q-InsOrd} \\ \midrule
			$\textsf{t-size}_{+}^{=1}$ & $\checkmark$  &   &   &   &   \\
			$\textsf{t-size}_{-}^{=1}$ & $\checkmark$  &   &   &   &   \\
			$\textsf{t-size}_{+}^{\leq 1}$ & $\checkmark$  &   &   &   &   \\
			$\textsf{t-size}_{-}^{\leq 1}$ & $\checkmark$  &   &   &   &   \\
			$\textsf{t-idx}_{+}$ &   &  $\checkmark$ &   &   &   \\
			$\textsf{t-idx}_{-}$ &   & $\checkmark$  &   &   &   \\
			$\textsf{t-val}_{+}$ &   &   &  $\checkmark$ &   &   \\
			$\textsf{t-val}_{-}$ &   &   & $\checkmark$  &   &   \\
			$\textsf{t-cor}_{+}^{b}$ &   &   &   & $\checkmark$  &   \\
			$\textsf{t-cor}_{-}^{b}$ &   &   &   &  $\checkmark$ &   \\
			$\textsf{t-cor}_{+}^{e}$ &   &   &   & $\checkmark$  &   \\
			$\textsf{t-cor}_{-}^{e}$ &   &   &   & $\checkmark$  &   \\
			$\ \textsf{t-cor}_{+}^{p}$ &   &   &   & $\checkmark$  &   \\
			$\textsf{t-cor}_{-}^{p}$ &   &   &   & $\checkmark$  &   \\
			$\textsf{t-cor}_{+}^{k}$ &   &   &   & $\checkmark$  &   \\
			$\textsf{t-cor}_{-}^{k}$ &   &   &   & $\checkmark$  &   \\
			$\textsf{t-InsOrd}_{+}$ &   &   &   &   &  $\checkmark$ \\
			$\textsf{t-InsOrd}_{-}$ &   &   &   &   &  $\checkmark$ \\ 
			\bottomrule
		\end{tabular}
	}
	\label{table:omega}
%%\vspace{-1mm} 
\end{table}

\subsection{Examples of Method Semantic Specification}
Table~\ref{table:semantic} presents the semantics of several methods of \textsf{ArrayList}, \textsf{HashSet}, and \textsf{LinkedHashMap} as examples.
For instance, the method \textsf{LinkedHashMap.put(O, O)} does not return any fact about the \textsf{LinkedHashMap} object and just modifies the object by adding a key-value pair.
The size will be increased by at most one.
Both the key and the value will belong to the \textsf{LinkedHashMap} object.
Meanwhile, the insertion order will be updated, and the key inserted by the method call will be set as the largest key.
Thus, it induces the container-property modifiers $\textsf{t-size}_{+}^{\leq 1}$, $\textsf{t-idx}_{+}$, $\textsf{t-val}_{+}$, $\textsf{t-cor}_{+}^{k}$, and $\textsf{t-InsOrd}_{+}$.

Consider the method \textsf{LinkedHashMap.containsKey(O)} as another example.
It does not modify the \textsf{LinkedHashMap} object and just returns the fact of whether the key has existed.
Therefore, it does not contain any container-property modifier and induces the container-property query $\textsf{q-isIdx}$.

We show examples to illustrate the form of the configurations in our implementation.
Several container methods are not listed in Table~\ref{table:semantic}, e.g., the methods \textsf{clear()} of the container types.
To describe the semantics of other methods, we need to add other queries and modifiers to $\mathcal{Q}$ and $\mathcal{T}$, respectively.
Obviously, it is trivial to write the semantic specifications for a given set of container types,
which does not demand any expertise knowledge.

\begin{table}[t]
	\centering
	\caption{Method Semantic Specification.}
	\resizebox{0.98\linewidth}{!} 
	{
		\begin{tabular}{c|c|l|l}
		\toprule
			Container	& Method	& $Q$ & $T$ \\ \midrule
			ArrayList	& add(O)	& $\varnothing$ & $\{ \textsf{t-size}_{+}^{=1}, \ \textsf{t-val}_{+}, \ \textsf{t-cor}_{+}^{e}\}$ \\
			ArrayList	& add(I, O)	& $\varnothing$ & $\{ \textsf{t-size}_{+}^{=1}, \ \textsf{t-val}_{+}, \ \textsf{t-cor}_{+}^{p}\}$ \\
			ArrayList	& contains(O)	& $\{\textsf{q-isVal}\}$ & $\varnothing$ \\
			ArrayList	& get(I)	& $\{\textsf{q-isCor}\}$ & $\varnothing$ \\
			ArrayList	& iterator()& $\{\textsf{q-size}, \ \textsf{q-isVal}, \ \textsf{q-isCor}\}$ & $\varnothing$\\
			ArrayList	& remove(I)	& $\varnothing$ & $\{ \textsf{t-size}_{-}^{=1}, \ \textsf{t-val}_{-}, \ \textsf{t-cor}_{-}^{p}\}$ \\
			ArrayList	& size()	& $\{\textsf{q-size}\}$ & $\varnothing$ \\ \hline
			HashSet	& add(O)	& $\varnothing$ & $\{ \textsf{t-size}_{+}^{\leq 1}, \ \textsf{t-val}_{+}\}$ \\
			HashSet	& contains(O)	& $\{\textsf{q-isVal}\}$ & $\varnothing$ \\
			HashSet	& iterator()& $\{\textsf{q-size}, \ \textsf{q-isVal}\}$ & $\varnothing$\\
			HashSet	& remove(O)	& $\varnothing$ & $\{ \textsf{t-size}_{-}^{\leq 1}, \ \textsf{t-val}_{-}\}$ \\
			HashSet	& size()	& $\{\textsf{q-size}\}$ & $\varnothing$ \\ \hline
			LinkedHashMap	& containsKey(O)	& $\{\textsf{q-isIdx}\}$ & $\varnothing$ \\
			LinkedHashMap	& containsValue(O)	& $\{\textsf{q-isVal}\}$ & $\varnothing$ \\
			LinkedHashMap	& get(O)	& $\{\textsf{q-isCor}\}$ & $\varnothing$ \\
			LinkedHashMap	& keySet()	& $\{\textsf{q-isIdx}\}$ & $\varnothing$ \\
			LinkedHashMap	& iterator()& $\{\textsf{q-size}, \ \textsf{q-isVal}, \ \textsf{q-isCor},\ \textsf{q-InsOrd}\}$ & $\varnothing$\\
			LinkedHashMap	& put(O, O)	& $\varnothing$ & $\{ \textsf{t-size}_{+}^{\leq 1}, \ \textsf{t-idx}_{+}, \ \textsf{t-val}_{+}, \ \textsf{t-cor}_{+}^{k}, \ \textsf{t-InsOrd}_{+}\}$ \\
			LinkedHashMap	& remove(O)	& $\varnothing$ & $\{ \textsf{t-size}_{-}^{\leq1}, \ \textsf{t-idx}_{-}, \ \textsf{t-val}_{-}, \ \textsf{t-cor}_{-}^{k}, \ \textsf{t-InsOrd}_{-}\}$ \\
			LinkedHashMap	& size()	& $\{\textsf{q-size}\}$ & $\varnothing$ \\ 
			LinkedHashMap	& values()	& $\{\textsf{q-isVal}\}$ & $\varnothing$ \\
		\bottomrule
		\end{tabular}
	}
	\label{table:semantic}
%	%\vspace{-1mm} 
\end{table}

\section{Method Complexity Specification}
We consider four container types as examples, including \textsf{ArrayList}, \textsf{HashSet}, \textsf{LinkedHashSet}, and \textsf{TreeSet}.

\subsection{Complexity Function}
\begin{table}[t]
	\centering
	\caption{Examples of Complexity Functions}
	\resizebox{0.98\linewidth}{!} 
	{
		\begin{tabular}{l|ccccccc}
		\toprule
			Complexity          & constant & \begin{tabular}[c]{@{}l@{}}amortized \\  \ constant\end{tabular} & logarithmic & \begin{tabular}[c]{@{}l@{}}\ amortized \\ logarithmic\end{tabular} & linear & \begin{tabular}[c]{@{}l@{}}amortized \\\ \ linear\end{tabular} & \begin{tabular}[c]{@{}l@{}}super\\ linear\end{tabular} \\ \midrule
			Complexity Function & $tc_1(n) = 1$ &  $tc_2(n)$ & $tc_3(n)=log\ n$ & $tc_4(n)$ & $tc_5(n) = n$& $tc_6(n)$ & $tc_7(n)$\\ 
					\bottomrule
		\end{tabular}
	}
	\label{table:complexitybasis}
%	%\vspace{-1mm} 
\end{table}

  \begin{table}
  	\caption{Method Complexity Specification}
  	\label{table:complexity}
  	%\vspace{-3mm}
	\begin{minipage}{0.49\linewidth}
		\resizebox{0.8\linewidth}{!} 
		{
			\begin{subtable}[t]{\linewidth}
				\caption*{}
				\begin{tabular}{c|c|c|c}
				\toprule
					Container	& Method	& Complexity Function & $\theta$ \\ \midrule
					ArrayList	& add(O)	& $tc_2(n)$ & 1\\
					ArrayList	& add(I, O)	& $tc_2(n)$ & 2\\
					ArrayList	& contains(O) & $tc_5(n)$ & 1\\
					ArrayList	& get(I)	& $tc_1(n)$ & 1\\
					ArrayList	& iterator()& $tc_1(n)$ & 1\\
					ArrayList	& remove(I)	& $tc_1(n)$ & 2\\
					ArrayList	& size()	&$tc_1(n)$ & 1\\ 		\bottomrule
				\end{tabular}
			
				%\vspace{5mm}
				
				\begin{tabular}{c|c|c|c}
				\toprule
					Container	& Method	& Complexity Function & $\theta$ \\ \midrule
					LinkedHashSet	& add(O)	& $tc_2(n)$ & 3\\
					LinkedHashSet	& contains(O) & $tc_1(n)$ & 1\\
					LinkedHashSet	& iterator() & $tc_1(n)$ & 1\\
					LinkedHashSet	& remove(O)	& $tc_2(n)$ & 3\\
					LinkedHashSet	& size() &	$tc_1(n)$ & 1\\ 		\bottomrule
				\end{tabular}
			\end{subtable}
		}
	\end{minipage}
	\begin{minipage}{0.49\linewidth}
		\resizebox{0.8\linewidth}{!} 
		{
			\begin{subtable}[t]{\linewidth}
				\centering
				\caption*{}
				\begin{tabular}{c|c|c|c}
					\toprule
					Container	& Method	& Complexity Function & $\theta$ \\ \midrule
					HashSet	& add(O)	& $tc_2(n)$ & 2\\
					HashSet	& contains(O) & $tc_1(n)$ & 1\\
					HashSet	& iterator()& $tc_1(n)$ & 1\\
					HashSet	& remove(O)	& $tc_2(n)$ & 2\\
					HashSet	& size() &	$tc_1(n)$ & 1\\ 		\bottomrule
				\end{tabular}
			
				%\vspace{13.5mm}
				
				\begin{tabular}{c|c|c|c}
					\toprule
					Container	& Method	& Complexity Function & $\theta$ \\ \midrule
					TreeSet	& add(O)	& $tc_3(n)$ & 2\\
					TreeSet	& contains(O)	& $tc_3(n)$ & 1\\
					TreeSet	& iterator() & $tc_1(n)$ & 1\\
					TreeSet	& remove(O)	& $tc_3(n)$ & 2\\
					TreeSet	& size()	&	$tc_1(n)$ & 1\\ 		\bottomrule
				\end{tabular}
			\end{subtable}
		}
	\end{minipage}
\end{table}

%\wcp{Add the order between the container method}
%\wcp{Add the complexity specification of LinkedList}
We select the complexity functions shown in Table~\ref{table:complexitybasis} to express method complexity specifications by adding factors to one of them.
The complexity functions of constant, logarithmic, and linear-complexity can be defined explicitly.
To represent the amortized complexity, we introduce $tc_2$, $tc_4$, and $tc_6$ symbolically without defining them explicitly.
Because any container method does not run in the time complexity higher than linear complexity,
we simply utilize $tc_7$ to represent all the complexity functions larger than a linear one.
By introducing the notations, we can describe the fact that 
the container method $f_{\mathcal{C}}$ with $tc_i$ as its complexity function consumes less time than the container method $g_{\mathcal{C}}$ with $c_j$ as its complexity function
if $i$ is smaller than $j$.

\subsection{Examples of Method Complexity Specification}
Table~\ref{table:complexity} shows the specifications of several methods of the four container types as examples.
We set $\theta$ to be a positive integer for each method so that the difference between the methods with the same complexity can be specified.
For example, the method \textsf{ArrayList.add(I, O)} consumes more time than the method \textsf{ArrayList.add(O)} 
because it has to shift the elements stored after the insertion position to the next slots.
We describe such difference by setting $\theta$ to 2 and 1 for the two methods, respectively.
Similarly, the methods \textsf{LinkedHashMap.add(O)} and \textsf{LinkedHashMap.remove(O)} have to update the linked list to maintain the insertion order,
and consume more time than the corresponding methods of \textsf{HashMap}.
Therefore, we set $\theta$ to 3 for \textsf{LinkedHashMap.add(O)} and \textsf{LinkedHashMap.remove(O)}, and 2 for \textsf{HashMap.add(O)} and \textsf{HashMap.remove(O)}.
Another point is the difference among the methods \textsf{contains(O)}, \textsf{add(O)} and \textsf{remove(O)} in \textsf{HashMap} and \textsf{LinkedHashMap}.
Although all of them run in amortized time complexity, the methods \textsf{add(O)} and \textsf{remove(O)} have to update the map objects by reorganizing hashing structure, 
and consume more time than the method \textsf{contains(O)}.
Therefore, we enforce $\theta$ of the methods \textsf{add(O)} and \textsf{remove(O)} larger than the one of \textsf{contains(O)}.
